# Supplementary material for: HyperNeRF: A Higher-Dimensional Representation for Topologically Varying Neural Radiance Fields
Source: arXiv:2106.13228 source file (2021-09-10)
Supplement: Supplementary file 1 [file interp_table_contents_combined.tex]

%%%% AUTOMATICALLY GENERATED, DO NOT EDIT.

\begin{tabular}{l||ccc|ccc|ccc|ccc|ccc|ccc|ccc|ccc|ccc|ccc}

\toprule
% Table Header (datasets).
& \multicolumn{ 3 }{c}{
  \makecell{
  \textsc{\small Expressions 1 }
\\(391 images)
  }
}
& \multicolumn{ 3 }{c}{
  \makecell{
  \textsc{\small Expressions 2 }
\\(126 images)
  }
}
& \multicolumn{ 3 }{c}{
  \makecell{
  \textsc{\small Expressions 3 }
\\(110 images)
  }
}
& \multicolumn{ 3 }{c}{
  \makecell{
  \textsc{\small Teapots }
\\(243 images)
  }
}
& \multicolumn{ 3 }{c}{
  \makecell{
  \textsc{\small Chicken }
\\(113 images)
  }
}
& \multicolumn{ 3 }{c}{
  \makecell{
  \textsc{\small Fist }
\\(433 images)
  }
}
& \multicolumn{ 3 }{c}{
  \makecell{
  \textsc{\small Slice Banana }
\\(82 images)
  }
}
& \multicolumn{ 3 }{c}{
  \makecell{
  \textsc{\small Torch }
\\(173 images)
  }
}
& \multicolumn{ 3 }{c}{
  \makecell{
  \textsc{\small Lemon }
\\(415 images)
  }
}
& \multicolumn{ 3 }{c}{
  \makecell{
  \textsc{\small Mean }
  }
}
\\

% Table header (metrics).
& \multicolumn{1}{c}{ \footnotesize PSNR$\uparrow$ }
& \multicolumn{1}{c}{ \footnotesize MS-SSIM$\uparrow$ }
& \multicolumn{1}{c}{ \footnotesize LPIPS$\downarrow$ }
& \multicolumn{1}{c}{ \footnotesize PSNR$\uparrow$ }
& \multicolumn{1}{c}{ \footnotesize MS-SSIM$\uparrow$ }
& \multicolumn{1}{c}{ \footnotesize LPIPS$\downarrow$ }
& \multicolumn{1}{c}{ \footnotesize PSNR$\uparrow$ }
& \multicolumn{1}{c}{ \footnotesize MS-SSIM$\uparrow$ }
& \multicolumn{1}{c}{ \footnotesize LPIPS$\downarrow$ }
& \multicolumn{1}{c}{ \footnotesize PSNR$\uparrow$ }
& \multicolumn{1}{c}{ \footnotesize MS-SSIM$\uparrow$ }
& \multicolumn{1}{c}{ \footnotesize LPIPS$\downarrow$ }
& \multicolumn{1}{c}{ \footnotesize PSNR$\uparrow$ }
& \multicolumn{1}{c}{ \footnotesize MS-SSIM$\uparrow$ }
& \multicolumn{1}{c}{ \footnotesize LPIPS$\downarrow$ }
& \multicolumn{1}{c}{ \footnotesize PSNR$\uparrow$ }
& \multicolumn{1}{c}{ \footnotesize MS-SSIM$\uparrow$ }
& \multicolumn{1}{c}{ \footnotesize LPIPS$\downarrow$ }
& \multicolumn{1}{c}{ \footnotesize PSNR$\uparrow$ }
& \multicolumn{1}{c}{ \footnotesize MS-SSIM$\uparrow$ }
& \multicolumn{1}{c}{ \footnotesize LPIPS$\downarrow$ }
& \multicolumn{1}{c}{ \footnotesize PSNR$\uparrow$ }
& \multicolumn{1}{c}{ \footnotesize MS-SSIM$\uparrow$ }
& \multicolumn{1}{c}{ \footnotesize LPIPS$\downarrow$ }
& \multicolumn{1}{c}{ \footnotesize PSNR$\uparrow$ }
& \multicolumn{1}{c}{ \footnotesize MS-SSIM$\uparrow$ }
& \multicolumn{1}{c}{ \footnotesize LPIPS$\downarrow$ }
& \multicolumn{1}{c}{ \footnotesize PSNR$\uparrow$ }
& \multicolumn{1}{c}{ \footnotesize MS-SSIM$\uparrow$ }
& \multicolumn{1}{c}{ \footnotesize LPIPS$\downarrow$ }
\\
\hline

% Table contents.
  NeRF~\cite{mildenhall2020nerf}
  &$21.6$
  &$.708$
  &$.582$
  
  &$21.1$
  &$.722$
  &$.492$
  
  &$15.6$
  &$.449$
  &$.747$
  
  &$23.6$
  &$.875$
  &$.339$
  
  &$18.8$
  &$.761$
  &$.453$
  
  &$23.8$
  &$.773$
  &$.469$
  
  &$20.8$
  &$.721$
  &$.513$
  
  &$22.5$
  &$.866$
  &$.373$
  
  &$24.1$
  &$.826$
  &$.437$
  
  &$21.3$
  &$.745$
  &$.490$
  
  \\   NV~\cite{lombardi2019neural}
  &$26.7$
  &\tablefirst$.900$
  &\tablefirst$.215$
  
  &$25.6$
  &$.910$
  &$.130$
  
  &$18.6$
  &$.647$
  &$.318$
  
  &$26.2$
  &$.917$
  &$.216$
  
  &$22.6$
  &$.861$
  &$.243$
  
  &$29.3$
  &$.912$
  &$.213$
  
  &$24.8$
  &$.907$
  &\tablethird$.209$
  
  &$24.6$
  &$.917$
  &$.189$
  
  &$28.8$
  &\tablethird$.951$
  &\tablefirst$.190$
  
  &$25.3$
  &$.880$
  &$.214$
  
  \\   NSFF~\cite{li2020nsff}
  &$26.6$
  &$.885$
  &$.283$
  
  &$29.8$
  &$.933$
  &$.134$
  
  &$18.3$
  &$.654$
  &$.317$
  
  &$25.8$
  &$.915$
  &\tablefirst$.210$
  
  &$27.7$
  &$.939$
  &$.173$
  
  &$24.9$
  &$.797$
  &$.329$
  
  &$26.1$
  &$.858$
  &$.243$
  
  &$22.3$
  &$.883$
  &$.253$
  
  &$28.0$
  &$.904$
  &$.238$
  
  &$25.5$
  &$.863$
  &$.242$
  
  \\   Nerfies~\cite{park2020nerfies}
  &$27.5$
  &$.877$
  &$.224$
  
  &$31.6$
  &$.963$
  &$.0952$
  
  &$19.7$
  &$.698$
  &\tablethird$.275$
  
  &$25.7$
  &$.922$
  &$.225$
  
  &$28.7$
  &\tablethird$.948$
  &\tablefirst$.141$
  
  &$29.9$
  &$.940$
  &$.171$
  
  &$27.9$
  &$.916$
  &$.209$
  
  &$27.8$
  &$.959$
  &\tablesecond$.169$
  
  &$30.8$
  &$.946$
  &\tablethird$.223$
  
  &$27.7$
  &$.908$
  &\tablesecond$.193$
  
  \\   Nerfies (w/o elastic)
  &$27.7$
  &$.883$
  &\tablethird$.219$
  
  &\tablethird$32.5$
  &\tablethird$.967$
  &\tablesecond$.0857$
  
  &\tablethird$20.0$
  &$.698$
  &$.279$
  
  &$25.8$
  &$.920$
  &$.229$
  
  &\tablethird$28.8$
  &$.947$
  &$.160$
  
  &\tablethird$30.5$
  &\tablethird$.946$
  &\tablethird$.158$
  
  &$28.1$
  &$.915$
  &\tablesecond$.200$
  
  &\tablethird$27.9$
  &\tablesecond$.961$
  &\tablefirst$.168$
  
  &$30.8$
  &$.946$
  &$.239$
  
  &$28.0$
  &$.909$
  &\tablethird$.193$
  
  \\ \hline  Hyper-NeRF (DS)
  &\tablesecond$27.9$
  &\tablesecond$.887$
  &\tablesecond$.218$
  
  &\tablesecond$32.9$
  &\tablefirst$.970$
  &\tablefirst$.0825$
  
  &\tablefirst$20.1$
  &\tablesecond$.703$
  &\tablesecond$.274$
  
  &\tablesecond$26.4$
  &\tablesecond$.931$
  &\tablesecond$.212$
  
  &$28.7$
  &$.948$
  &\tablethird$.156$
  
  &\tablefirst$30.7$
  &\tablefirst$.950$
  &\tablefirst$.150$
  
  &\tablefirst$28.4$
  &\tablefirst$.920$
  &\tablefirst$.191$
  
  &\tablesecond$28.0$
  &\tablefirst$.962$
  &\tablethird$.172$
  
  &\tablefirst$31.8$
  &\tablefirst$.956$
  &\tablesecond$.210$
  
  &\tablefirst$28.3$
  &\tablefirst$.914$
  &\tablefirst$.185$
  
  \\   Hyper-NeRF (DS, w/ elastic)
  &\tablethird$27.8$
  &$.885$
  &$.220$
  
  &$32.4$
  &$.966$
  &$.0956$
  
  &$19.9$
  &\tablethird$.700$
  &\tablefirst$.269$
  
  &\tablefirst$26.4$
  &\tablefirst$.932$
  &\tablethird$.212$
  
  &\tablesecond$28.8$
  &\tablefirst$.949$
  &\tablesecond$.145$
  
  &$30.2$
  &$.943$
  &$.162$
  
  &\tablethird$28.3$
  &\tablesecond$.918$
  &$.249$
  
  &$27.9$
  &$.960$
  &$.173$
  
  &\tablesecond$31.4$
  &\tablesecond$.952$
  &$.230$
  
  &\tablethird$28.1$
  &\tablethird$.912$
  &$.195$
  
  \\   Hyper-NeRF (AP)
  &\tablefirst$27.9$
  &\tablethird$.885$
  &$.240$
  
  &\tablefirst$33.1$
  &\tablesecond$.970$
  &\tablethird$.0894$
  
  &\tablesecond$20.0$
  &\tablefirst$.703$
  &$.290$
  
  &\tablethird$26.3$
  &\tablethird$.927$
  &$.234$
  
  &\tablefirst$28.9$
  &\tablesecond$.949$
  &$.162$
  
  &\tablesecond$30.5$
  &\tablesecond$.947$
  &\tablesecond$.158$
  
  &\tablesecond$28.4$
  &\tablethird$.917$
  &$.241$
  
  &\tablefirst$28.0$
  &\tablethird$.960$
  &$.183$
  
  &\tablethird$31.3$
  &$.947$
  &$.276$
  
  &\tablesecond$28.3$
  &\tablesecond$.912$
  &$.208$
  
  \\   Hyper-NeRF (w/o deform)
  &$26.9$
  &$.857$
  &$.312$
  
  &$31.1$
  &$.947$
  &$.131$
  
  &$19.4$
  &$.669$
  &$.352$
  
  &$26.0$
  &$.922$
  &$.238$
  
  &$27.7$
  &$.936$
  &$.203$
  
  &$29.3$
  &$.924$
  &$.212$
  
  &$28.1$
  &$.915$
  &$.299$
  
  &$27.3$
  &$.951$
  &$.224$
  
  &$30.5$
  &$.937$
  &$.303$
  
  &$27.4$
  &$.895$
  &$.253$
  
  \\ \bottomrule

\end{tabular}

%%%% AUTOMATICALLY GENERATED, DO NOT EDIT.
